# Supplementary material for: BANER: Boundary-Aware LLMs for Few-Shot Named Entity Recognition
Source: arXiv:2412.02228 source file (2024-12-03)
Supplement: Supplementary file 1 [file appendix.tex]

\appendix
\section{Appendix}

\subsection{Target Domain Inference Algorithm}\label{app:algorithm_1}

Algorithm~\ref{algorithm_1} describes the process of domain adaptation using support set in the target domain and prediction on the query set.
Lines 1-7 describe the target domain adaptation process for the span detection stage.
Lines 8-14 describe the target domain adaptation process for the type classification stage.
Lines 15-19 describe the extraction of candidate entity spans in the query set using the fine-tuned span detector.
Lines 20-31 describe the candidate entity span filtering and entity type classification using type-aware prototypes.

\begin{algorithm}[t]
\begin{footnotesize}
\caption{Procedure of target domain inference in \ours .}
\begin{algorithmic}[1]\label{algorithm_1}
 \REQUIRE{Support set $S_{target}$; Query set $Q_{target}$; Class set $\mathcal{T}_{target}$; Encoders $f_{\theta_1}$, $f_{\theta_2}$;}
 \ENSURE{Query set predictions $S_{result}$}

 \STATE {$\mathcal{L}_{prev} = \infty$; $\mathcal{L}_{prev} \in \mathbb{R}_{+}$ (Any large positive value);}\\
 
 \STATE {$\mathcal{L}_{span} = \mathcal{L}_{prev} - 1$;}
 
 \WHILE{$\mathcal{L}_{span} < \mathcal{L}_{prev}$}
     \STATE {$\mathcal{L}_{prev} = \mathcal{L}_{span}$;}\\
     \STATE {Compute loss $\mathcal{L}_{span}$ using Eq. (\ref{loss_span_detector});}\\
     \STATE {Update $f_{\theta_2} \rightarrow f_{\theta_2^{'}}$ to reduce $\mathcal{L}_{span}$;}\\
     
 \ENDWHILE \\
 
 \STATE {$\mathcal{L}_{prev} = \infty$; $\mathcal{L}_{prev} \in \mathbb{R}_{+}$ (Any large positive value);}
 \STATE {$\mathcal{L}_{label} = \mathcal{L}_{prev} - 1$;}
 \WHILE{$\mathcal{L}_{label} < \mathcal{L}_{prev}$}
     \STATE {$\mathcal{L}_{prev} = \mathcal{L}_{label}$;}
     \STATE {Compute loss $\mathcal{L}_{label}$ using Eq. (\ref{eq_entity_label_loss});}
     \STATE {Update parameters ${\theta_2} \rightarrow {\theta_2^{'}}$ to reduce $\mathcal{L}_{label}$;}
 \ENDWHILE \\
 
\STATE {$C_{span} = \{\}$;}
\FOR{$X_i$ in $Q_{target}$}
    \STATE {Extract candidate entity spans $C_{span}^{i}$ from sentence $X_i$ according to Section~\ref{early_stopping_span};}\\
    \STATE {$C_{span} = C_{span} \cup C_{span}^{i}$;}\\
\ENDFOR

\STATE {Calculate threshold $\gamma_{t}$ for span filtering using Eq. (\ref{gamma_t});}\\
\STATE {Calculate all prototypes in $\mathcal{T}_{target}$ using Eq. (\ref{inferece_prototype});}\\
\STATE {The prototype of class $t_j$ is denoted as $\mathbf{p_j}$};\\

{$S_{result} = \{\}$;}
\FOR{$s_i$ in $C_{span}$}
    \STATE {$max\_sim = \max\limits_{t_j \in \mathcal{T}_{target}}((f_{\theta_2^{'}}(s_i) \oplus f_{\theta_2^{'}}(s_i)) \cdot \mathbf{p_j}^{\mathsf{T}})$}
    \IF{$max\_sim/2 > \gamma_{t}$}
        \STATE {Assign the label $y_{pred}$ to $s_{i}$ using Eq. (\ref{eq_final_inference});}\\
        \STATE {$S_{result}$ = $S_{result}$ $\cup$ \{$s_{i}$\};}\\
    \ELSE
        \STATE {Remove this candidate span $s_{i}$;}\\
    \ENDIF
\ENDFOR

\end{algorithmic}
\end{footnotesize}
\end{algorithm}

\subsection{Details of Datasets and Evaluation Methods}\label{appendix_datasets}
\subsubsection{Statistics of Datasets}
Table \ref{tab:dataset-statistic} shows statistics of various datasets used in our experiments.

\begin{table}[htb]
    \centering
    \small
    \resizebox{\columnwidth}{!}{
        \begin{tabular}{ccccc}
        \toprule
           \textbf{Dataset}  & \textbf{Domain} & \textbf{\# Classes}& \textbf{\# Sentences}  & \textbf{\# Entities} \\
           \cmidrule(r){1-1} \cmidrule(r){2-5} 
         % \midrule
           Few-NERD  & Wikipedia & 66& 188.2k  &491.7k\\
           I2B2'14 & Medical & 23& 140.8k  &29.2k\\
           CoNLL'03 & News & 4& 20.7k  &35.1k\\
           GUM & Wiki & 11& 3.5k  &6.1k\\
           WNUT'17 & Social  & 6 & 5.7k &3.9k\\
           OntoNotes & General & 18 & 76.7k &104.2k\\
         \bottomrule
        \end{tabular}
    }
    \caption{Dataset statistics}
    \label{tab:dataset-statistic}
\end{table}

\subsubsection{Evaluation Methods}
\paragraph{Episode-level Evaluation}
Following~\citet{ma-etal-2022-decomposed}, we adopt the episode-level evaluation method for Few-NERD settings. 
Each episode consists of a support set and a query set, both given in the n-way k-shot form. 
In each episode, the model trained in the source domain is tested on the query set by utilizing the support set. 
To make fair comparisons, we obtain the Micro F1 score with the episode-data processed by~\citet{ding2021few}. 
We report the mean F1 score with standard deviation using 3 different seeds.

\paragraph{Dataset-level Evaluation}
\citet{yang-katiyar-2020-simple} point that sampling test episodes may not reflect the real-world performance due to various data distributions, and they propose to sample support sets and then test the model in the original test set.
Each support set consists of $k$ examples corresponding to each label.
The final Micro F1 scores and standard deviations are obtained using different sampled support sets.
Thus, following~\citet{yang-katiyar-2020-simple} and~\citet{das-etal-2022-container}, we also adopt this evaluation schema for {Domain Transfer} settings.

\subsection{Baselines}\label{appendix_baselines}
{\textbf{ProtoBERT}~\cite{fritzler-2019}} adopts a token-level prototypical network, where the prototype of each class is obtained by averaging token samples of the same label, and the label of each unlabeled token in the query set is determined by its nearest class prototype.\\
{\textbf{NNShot}~\cite{yang-katiyar-2020-simple}} pre-trains BERT by traditional classification methods in the source domain training phase, and decides the class of each unlabeled token by the nearest neighbor at the token level in the target domain inference phase.\\
{\textbf{StructShot}~\cite{yang-katiyar-2020-simple}} is based on NNshot and uses an abstract transition probability for Viterbi decoding during testing.\\
{\textbf{ESD}~\cite{wang-2022-enhanced}} uses a span-level prototypical network, which designs multiple prototypes for \nonetoken-tokens and uses inter- and cross-span attention for better span representation.\\
{\textbf{FSLS}~\cite{ma2022label}} adopts two encoders, one for obtaining type names representations and the other for token representations.  
During the training procedure, the Euclidean distance between tokens and their corresponding type name semantics are minimized.
During prediction, the label for a token is determined based on the closest type name semantics.
We chose this baseline to demonstrate the superiority of our approach over existing approaches using the semantics of type names.\\
{\textbf{CONTaiNER}~\cite{das-etal-2022-container}} first trains BERT in the source domain using token-level contrastive learning loss function, then fine-tunes the trained model on the support set, and finally use the nearest neighbor method proposed in NNShot~\cite{yang-katiyar-2020-simple} for target domain inference phase.\\
{\textbf{DecomposedMetaNER}~\cite{ma-etal-2022-decomposed}} is a decomposed approach that incorporates model-agnostic meta-learning strategy into traditional prototypical network to learn a model-agnostic model and more fully exploits the support set.\\

\subsection{Implementation Details}\label{appendix_implementation_details}
Following previous methods~\cite{ding2021few,das-etal-2022-container,ma-etal-2022-decomposed}, we use {\texttt{bert-base-uncased}} model~\cite{devlin-etal-2019-bert} from HuggingFace~\cite{wolf-etal-2020-transformers}\footnote{\url{https://huggingface.co/bert-base-uncased}} as our encoder $f_{\theta_1}$ and $f_{\theta_2}$.

During the source domain training procedure, we use AdamW~\cite{loshchilov2018decoupled} as the optimizer with a learning rate of 3e-5 and 1\% linear warmup steps, and the batch size is set to 64. We set the temperature hyper-parameter $\tau$ = 0.05 in Eq.(\ref{loss_type_contrastive_loss}) and keep dropout rate as 0.2 in the classification layer of the span detection.

As for the early stopping strategy in \ref{early_stopping_span}, we found that the fewer samples face a higher risk of over-fitting, and a lower $\beta$ threshold is required. So we set $\beta$ = 2 in all 1-shot settings and $\beta$ = 6 in all other cases.
Table \ref{tab:hyper-parameters} shows the searching space of each hyper-parameter. Besides, we implement our framework with Pytorch 1.12\footnote{\url{https://pytorch.org/}} and train it with a V100-16G GPU.

Using a V100-16G GPU, we trained the model on the source domain OntoNotes dataset for 60 minutes. 
The finetuning procedures of span detection and type classification stages require less than 20 seconds in total under 5-shot settings.

\begin{table}[htb]
    \centering
    \small
    {
        \begin{tabular}{lc}
        \toprule
            Learning rate & \{1e-5, 3e-5, 1e-4\} \\
            Batch size & \{ 32, 64, 128\} \\ 
            Dropout rate & \{0.1, 0.2, 0.5\} \\
            temperature $\tau$ & \{0.01, 0.05, 0.1\} \\
            Early stopping threshold $\beta$ & \{1, 2, 4, 6, 8\} \\
         \bottomrule
        \end{tabular}
    }
    \caption{Hyper-parameters search space in our experiments.}
    \label{tab:hyper-parameters}
\end{table}

\subsection{Analysis of Tagging Schemes in the Span Detection Stage}\label{appendix_results_span_detection}

\begin{table*}[htb]
    \centering
    \small
    \setlength{\tabcolsep}{1.2mm}
    \resizebox{\textwidth}{!}
    {
        \begin{tabular}{ccccccccccccccc}
        \toprule
        \multirow{3}{*}{\textbf{Stage}} & \multirow{3}{*}{\textbf{Filtered}}             & \multirow{3}{*}{\textbf{Schema}} & \multicolumn{6}{c}{\textbf{I2B2}}                             & \multicolumn{6}{c}{\textbf{CoNLL}}                            \\
        \cmidrule(lr){4-9} \cmidrule(lr){10-15} 
                                        &                                                &                                  & \multicolumn{3}{c}{1-shot}    & \multicolumn{3}{c}{5-shot}    & \multicolumn{3}{c}{1-shot}    & \multicolumn{3}{c}{5-shot}    \\
        \cmidrule(lr){4-6} \cmidrule(lr){7-9} \cmidrule(lr){10-12} \cmidrule(lr){13-15} 
                                        &                                                &                                  & Precision & Recall  & F1      & Precision & Recall  & F1      & Precision & Recall  & F1      & Precision & Recall  & F1      \\
        \cmidrule(lr){1-3} \cmidrule(lr){4-9} \cmidrule(lr){10-15} 
        \multirow{6}{*}{Span}           & \multirow{3}{*}{\textit{No}}  & IO                                                & 19.62   & 70.59 & 30.46 & 25.12   & 77.71 & 37.86 & 75.05   & 84.28 & 78.96 & 87.48   & 90.68 & 89.01 \\
                                        &                                                & BIO                              & 19.84   & 67.89 & 30.49 & 22.36   & 75.76 & 34.40 & 72.01   & 84.27 & 77.15 & 85.87   & 88.78 & 87.24 \\
                                        &                                                & BIOES                            & 19.71   & 60.46 & 29.47 & 23.89   & 70.19 & 35.53 & 70.38   & 80.93 & 74.89 & 84.02   & 87.77 & 85.72 \\
        \cmidrule(lr){2-2} \cmidrule(lr){3-3} \cmidrule(lr){4-9} \cmidrule(lr){10-15}
                                        & \multirow{3}{*}{\textit{Yes}} & IO                                                & 53.79   & 41.54 & 45.33 & 55.78   & 52.84 & 53.82 & 78.65   & 83.25 & 80.47 & 87.86   & 89.56 & 88.67 \\
                                        &                                                & BIO                              & 54.20   & 40.83 & 45.63 & 53.24   & 55.64 & 53.63 & 77.22   & 84.29 & 80.18 & 87.11   & 88.78 & 87.90 \\
                                        &                                                & BIOES                            & 52.77   & 34.04 & 39.80 & 57.46   & 50.97 & 53.32 & 74.39   & 80.72 & 77.00 & 84.65   & 87.65 & 86.00 \\
        \cmidrule(lr){1-3} \cmidrule(lr){4-9} \cmidrule(lr){10-15} 
        \multirow{6}{*}{Span+Type}      & \multirow{3}{*}{\textit{No}}  & IO                                                & 14.14   & 47.18 & 21.57 & 17.83   & 51.11 & 26.35 & 65.37   & 72.73 & 68.47 & 79.06   & 81.32 & 80.14 \\
                                        &                                                & BIO                              & 14.92   & 49.32 & 22.74 & 16.65   & 54.40 & 25.40 & 63.66   & 74.08 & 68.01 & 77.88   & 80.27 & 79.00 \\
                                        &                                                & BIOES                            & 14.18   & 42.01 & 21.02 & 17.44   & 49.36 & 25.69 & 61.84   & 70.69 & 65.62 & 76.36   & 79.46 & 77.75 \\
        \cmidrule(lr){2-2} \cmidrule(lr){3-3} \cmidrule(lr){4-9} \cmidrule(lr){10-15}
                                        & \multirow{3}{*}{\textit{Yes}} & IO                                                & 47.24   & 35.77 & 39.32 & 46.92   & 44.33 & 45.20 & 68.89   & 72.70 & 70.38 & 79.81   & 81.31 & 80.53 \\
                                        &                                                & BIO                              & 47.83   & 35.42 & 39.87 & 45.18   & 47.00 & 45.39 & 67.98   & 74.07 & 70.52 & 78.75   & 80.26 & 79.47 \\
                                        &                                                & BIOES                            & 45.47   & 28.69 & 33.80 & 47.54   & 42.15 & 44.10 & 65.26   & 70.62 & 67.46 & 76.80   & 79.46 & 77.99 \\
        \bottomrule
        \end{tabular}
    }
    \caption{span detection.}
    \label{tab:app_span_detection_1}
\end{table*}

\begin{table*}[htb]
    \centering
    \small
    \setlength{\tabcolsep}{1.2mm}
    \resizebox{\textwidth}{!}
    {
        \begin{tabular}{ccccccccccccccc}
        \toprule
        \multirow{3}{*}{\textbf{Stage}} & \multirow{3}{*}{\textbf{Filtered}}             & \multirow{3}{*}{\textbf{Schema}} & \multicolumn{6}{c}{\textbf{WNUT}}                             & \multicolumn{6}{c}{\textbf{GUM}}                            \\
        \cmidrule(lr){4-9} \cmidrule(lr){10-15} 
                                        &                                                &                                  & \multicolumn{3}{c}{1-shot}    & \multicolumn{3}{c}{5-shot}    & \multicolumn{3}{c}{1-shot}    & \multicolumn{3}{c}{5-shot}    \\
        \cmidrule(lr){4-6} \cmidrule(lr){7-9} \cmidrule(lr){10-12} \cmidrule(lr){13-15} 
                                        &                                                &                                  & Precision & Recall  & F1      & Precision & Recall  & F1      & Precision & Recall  & F1      & Precision & Recall  & F1      \\
        \cmidrule(lr){1-3} \cmidrule(lr){4-9} \cmidrule(lr){10-15} 
        \multirow{6}{*}{Span}           & \multirow{3}{*}{\textit{No}}  & IO                                                & 38.42              & 65.42              & 47.37              & 40.70              & 65.64              & 49.13              & 45.93              & 45.70              & 45.72              & 56.41              & 64.25              & 60.04              \\
                                        &                                                & BIO                              & 40.89              & 63.85              & 48.82              & 38.28              & 68.60              & 48.92              & 44.86              & 45.67              & 45.05              & 53.99              & 64.34              & 58.64              \\
                                        &                                                & BIOES                            & 42.67              & 56.14              & 47.30              & 41.90              & 65.24              & 50.59              & 54.28              & 48.32              & 50.97              & 60.57              & 64.07              & 62.22              \\
        \cmidrule(lr){2-2} \cmidrule(lr){3-3} \cmidrule(lr){4-9} \cmidrule(lr){10-15}
                                        & \multirow{3}{*}{\textit{Yes}} & IO                                                & 40.86              & 63.50              & 48.49              & 41.13              & 65.27              & 49.34              & 46.14              & 44.61              & 45.26              & 55.98              & 62.09              & 58.84              \\
                                        &                                                & BIO                              & 43.61              & 61.33              & 49.41              & 38.74              & 68.15              & 49.17              & 45.55              & 45.74              & 45.44              & 54.74              & 64.40              & 59.11              \\
                                        &                                                & BIOES                            & 45.78              & 54.39              & 48.14              & 42.45              & 65.06              & 50.92              & 54.58              & 47.92              & 50.88              & 60.88              & 63.56              & 62.15              \\
        \cmidrule(lr){1-3} \cmidrule(lr){4-9} \cmidrule(lr){10-15} 
        \multirow{6}{*}{Span+Type}      & \multirow{3}{*}{\textit{No}}  & IO                                                & 25.86              & 43.19              & 31.62              & 28.59              & 45.35              & 34.26              & 24.64              & 23.90              & 24.21              & 33.39              & 37.02              & 35.09              \\
                                        &                                                & BIO                              & 27.34              & 42.11              & 32.52              & 25.69              & 45.83              & 32.77              & 24.97              & 25.24              & 24.99              & 33.14              & 39.04              & 35.81              \\
                                        &                                                & BIOES                            & 28.94              & 36.92              & 31.74              & 28.60              & 44.37              & 34.48              & 30.20              & 26.65              & 28.23              & 37.38              & 39.02              & 38.15              \\
        \cmidrule(lr){2-2} \cmidrule(lr){3-3} \cmidrule(lr){4-9} \cmidrule(lr){10-15}
                                        & \multirow{3}{*}{\textit{Yes}} & IO                                                & 27.95              & 42.60              & 32.84              & 28.95              & 45.34              & 34.51              & 24.65              & 23.87              & 24.20              & 33.39              & 37.02              & 35.09              \\
                                        &                                                & BIO                              & 29.79              & 41.22              & 33.56              & 26.06              & 45.80              & 33.06              & 24.98              & 25.23              & 24.99              & 33.14              & 39.04              & 35.81              \\
                                        &                                                & BIOES                            & 31.72              & 36.31              & 32.85              & 28.95              & 44.37              & 34.72              & 30.21              & 26.64              & 28.22              & 37.38              & 39.02              & 38.15              \\
        \bottomrule
        \end{tabular}
    }
    \caption{span detection.}
    \label{tab:app_span_detection_2}
\end{table*}

Table~\ref{tab:app_span_detection_1} and Table~\ref{tab:app_span_detection_2} show the span detection and overall performance under the Domain Transfer settings.
We observe that: 
1) The three tagging schemes have their own advantages and disadvantages. IO and BIO schemes can achieve higher recall, BIOES can achieve higher precision. 
2) The IO tagging scheme can achieve the best overall performance in most settings, except for the GUM dataset. 
Therefore, the IO scheme is selected for the span detection stage in this paper.	
3) The type-aware span filtering strategy proposed in this paper shown robust and positive effects across different tagging schemes.
Even when dealing with entity-dense datasets, where incorrect entity spans are minimal, this strategy does not significantly impair performance.
In future work, we can try to combine the advantages and disadvantages of different tagging schemes to further improve the performance of the span detection stage.

\subsection{Case Study}
To examine how our model accurately constructs prototypes and filters out over-detected false spans  with the help of type names, we randomly select one query sentence from Few-NERD intra and CoNLL2003 for case study.
We compare \ours with DecomposedMetaNER~\cite{ma-etal-2022-decomposed}, which also belongs to the two-stage methods.\looseness=-1

\begin{figure*}[tbh!]
\vspace{-0mm}
\centering
\includegraphics[width=1.0\textwidth]{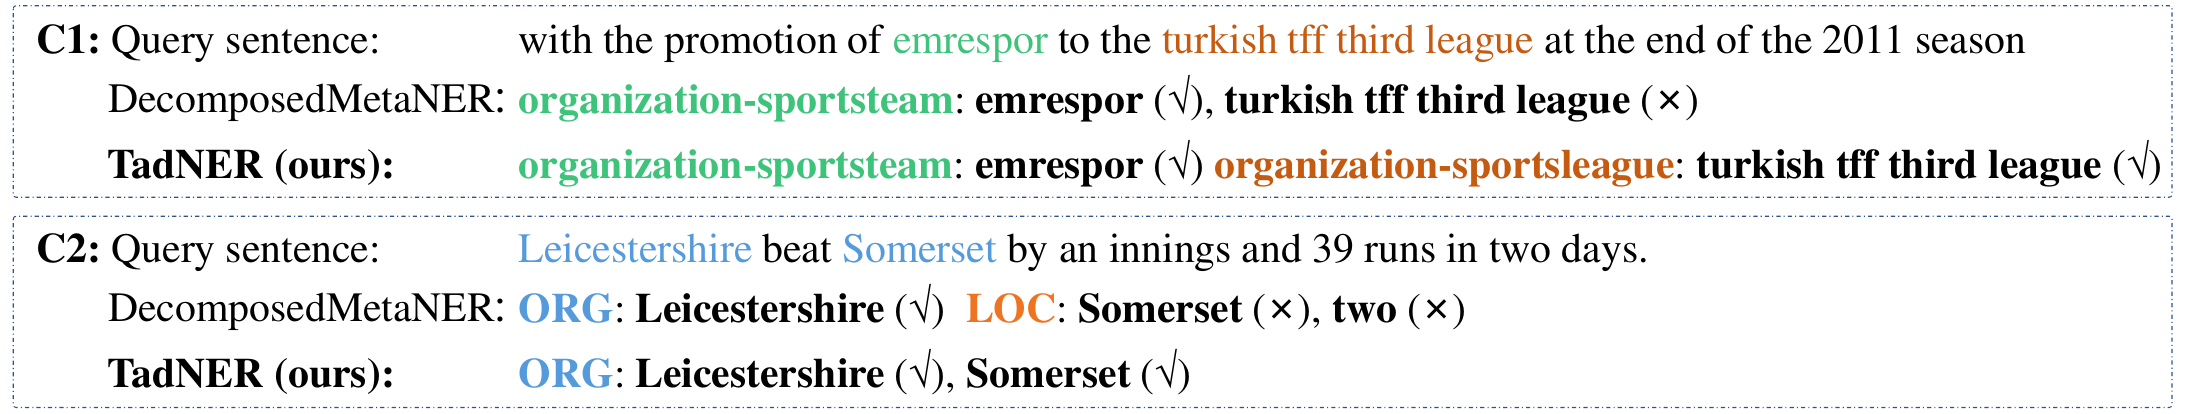}
\caption{Case study.
 C1 and C2 are from Few-NERD intra and CoNLL2003 in Cross datasets, respectively, and \textcolor[RGB]{0,176,80}{organization-sportsteam}, \textcolor[RGB]{197,90,17}{organization-sportsleague}, \textcolor[RGB]{114,172,225}{ORG} and \textcolor[RGB]{239,116,33}{LOC} are entity types.
}
\label{fig_case_study}
\vspace{-2mm}
\end{figure*}

As shown in Fig.~\ref{fig_case_study}, in the first case, our model correctly predicts ``turkish tff third league'' as ``organization-sportsleague'' type, while DecomposedMetaNER identifies it as a wrong ``organization-sportsteam'' type.
Since the type name and the entity span have a overlapping word ``league'', incorporating the type name into the construction of the prototype will make the identification much easier. Conversely, without the type name, it would be difficult to distinguish between two categories of entities because they both represent ``sports-related organizations''.

In the second case, DecomposedMetaNER incorrectly identifies ``two'' as an entity span and then assigns it a wrong entity type ``LOC'', since there are many samples like ``The two sides had not met since Oct. 18'' in the source domain Ontonotes, where ``two'' is an entity of ``CARDINAL'' type.
In contrast, our \ours removes this false span successfully by applying the  type-aware span filtering strategy. \looseness=-1

\subsection{Zero-Shot Performance}\label{appendix_zero}
Since there is no domain-specific support set under zero-shot NER settings, it is extremely challenging and rarely explored.
While we believe our proposed \ours can obtain certain zero-shot ability after training in the source doamin for the following two reasons: 1) the model can extract entity spans in the span detection stage before fine-tuning with support samples, 2) since the feature space learnt in the type classification stage is well generalized and type-aware, we can directly adopt the representations of type names as prototypes of novel entity types.
To demonstrate the promising performance of our model under zero-shot settings, we select SpanNER~\cite{wang2021learning-from-description} as a strong baseline, which is a decomposed-based method and good at solving zero-shot NER problem.

\begin{table}[htb]
    \small
    \centering
    \setlength{\tabcolsep}{1mm}  
    {
    \begin{tabular}{lcccccccc}
    \toprule
        \multirow{2}{*}{\textbf{Model}}  & \multicolumn{5}{c}{\textbf{Domain Transfer}}\\
        \cmidrule(lr){2-6} 
        & {I2B2} & {CoNLL}  & {WNUT} & {GUM} & {Avg.}\\
         \cmidrule(lr){1-1}\cmidrule(lr){2-6} 
        % ProtoBERT (1-shot) & 20.76 & 15.05 & 42.54 & 35.40 & 13.40 & 49.90  & 17.40 & 17.80\\

        SpanNER (0-shot)  & 8.02 & 23.63  & 24.82 & 6.57 & 15.76\\
        
        \textbf{\ours (0-shot)}  & \textbf{17.13}& \textbf{43.14} & \textbf{25.06}& \textbf{7.62} & \textbf{23.24}\\
        \bottomrule
    \end{tabular}
    }
    \caption{F1 scores under Domain Transfer zero-shot settings.}
    \label{tab:performance_zero_shot}
\end{table}

As shown in Table \ref{tab:performance_zero_shot}, our proposed \ours performs better than SpanNER~\cite{wang2021learning-from-description} under every case.
The reason for this may be that the type classification of SpanNER is based on a traditional supervised classification model, which performs worse generalization in cross-domain scenarios.
Besides, compared with previous metric-based methods~\cite{das-etal-2022-container,ma-etal-2022-decomposed} for few-shot NER, which heavily rely on support sets and had \textbf{no} zero-shot capability, our method is more inspirational for future zero-shot NER works.

\subsection{Detailed Type Names}

\subsubsection{Original Type Names}\label{appendix_type_names}

\begin{table}[H]
\small
\begin{center}
\resizebox{\columnwidth}{!}  {
\begin{tabular}{lcl}
\toprule
\bf Dataset & \makecell[c]{\textbf{Labels}} & \makecell[c]{\textbf{Type names}} \\

\cmidrule(lr){1-1} \cmidrule(lr){2-3}
\multirow{66}{*}{\textbf{Few-NERD} } 
    &art-broadcastprogram &  broadcast program \\
    &art-film & film \\
    &art-music & music \\
    &art-other & other art\\
    &art-painting & painting \\
    &art-writtenart & written art \\
    &person-actor & actor \\
    &person-artist/author & artist author \\
    &person-athlete & athlete \\
    &person-director & director \\
    &person-other & other person \\
    &person-politician & politician \\
    &person-scholar & scholar \\
    &person-soldier &  soldier \\ 
    &product-airplane & airplane \\
    &product-car &  car \\
    &product-food &  food \\ 
    &product-game & game \\
    &product-other &  other product \\ 
    &product-ship & ship \\
    &product-software &  software \\
    &product-train &  train \\
    &product-weapon &  weapon \\
    &other-astronomything & astronomy thing \\
    &other-award &  award \\
    &other-biologything &  biology thing \\ 
    &other-chemicalthing & chemical thing \\ 
    &other-currency & currency \\
    &other-disease &  disease \\
    &other-educationaldegree &  educational degree \\ 
    &other-god & god \\ 
    &other-language & language \\
    &other-law &  law \\
    &other-livingthing & living thing \\
    &other-medical & medical \\

    &building-airport & airport \\
    &building-hospital & hospital \\
    &building-hotel & hotel \\
    &building-library & library \\
    &building-other & other building \\
    &building-restaurant & restaurant \\
    &building-sportsfacility & sports facility \\
    &building-theater & theater \\
    &\makecell[c]{event-attack/battle\\/war/militaryconflict} & \makecell[l]{attack battle \\war military conflict} \\
    &event-disaster & disaster \\
    &event-election & election \\
    &event-other & other event \\
    &event-protest & protest \\
    &event-sportsevent & sports event \\
    &location-bodiesofwater & bodies of water \\
    &location-GPE & \makecell[l]{geographical social \\political entity} \\
    &location-island & island \\
    &location-mountain & mountain \\
    &location-other & other location \\
    &location-park & park \\
    &\makecell[c]{location-road/railway\\/highway/transit} & \makecell[l]{road railway \\highway transit} \\
    &organization-company & company \\
    &organization-education & education \\
    &\makecell[c]{organization-government\\/governmentagency} & government agency \\
    &organization-media/newspaper & media newspaper \\
    &organization-other & other organization \\
    &organization-politicalparty & political party \\
    &organization-religion & religion \\
    &organization-showorganization & show organization \\
    &organization-sportsleague & sports league \\
    &organization-sportsteam & sports team \\

\bottomrule
\end{tabular}

}

\end{center}
\caption{Original labels and their corresponding natural-language-form type names of {Few-NERD}.}
\label{tab:dataset_labels_nlf_1}
\end{table}

\begin{table}[H]
\small
\begin{center}
\resizebox{\columnwidth}{!} {
\begin{tabular}{lcl}
\toprule
\bf Dataset & \makecell[c]{\textbf{Labels}} & \makecell[c]{\textbf{Type names}} \\

\cmidrule(lr){1-1} \cmidrule(lr){2-3}
\multirow{23}{*}{\textbf{I2B2'14} } 
& AGE & age \\
& BIOID & biometric ID \\
& CITY & city \\
& COUNTRY & country \\
& DATE & date \\
& DEVICE & device \\
& DOCTOR & doctor \\
& EMAIL & email \\
& FAX & fax \\
& HEALTHPLAN & health plan number \\
& HOSPITAL & hospital \\
& IDNUM & ID number \\
& LOCATION\_OTHER & location \\
& MEDICALRECORD & medical record \\
& ORGANIZATION & organization \\
& PATIENT & patient \\
& PHONE & phone number \\
& PROFESSION & profession \\
& STATE & state \\
& STREET & street \\
& URL & url \\
& USERNAME & username \\
& ZIP & zip code \\

\cmidrule(lr){1-1} \cmidrule(lr){2-3}
\multirow{4}{*}{\textbf{CoNLL'03} } 
& PER & person \\
& LOC & location \\
& ORG & organization \\
& MISC & miscellaneous \\

\cmidrule(lr){1-1} \cmidrule(lr){2-3}
\multirow{11}{*}{\textbf{GUM} } 
& abstract & abstract \\
& animal & animal \\
& event & event \\
& object & object \\
& organization & organization \\
& person & person \\
& place & place \\
& plant & plant \\
& quantity & quantity \\
& substance & substance \\
& time & time \\

\cmidrule(lr){1-1} \cmidrule(lr){2-3}
\multirow{6}{*}{\textbf{WNUT'17} } 
& corporation & corporation \\
& creative-work & creative work \\
& group & group \\
& location & location \\
& person & person \\
& product & product \\

\cmidrule(lr){1-1} \cmidrule(lr){2-3}
\multirow{18}{*}{\textbf{Ontonotes} } 
& CARDINAL & cardinal \\
& DATE & date \\
& EVENT & event \\
& FAC & fac \\
& GPE & \makecell[l]{geographical social \\political entity} \\
& LANGUAGE & language \\
& LAW & law \\
& LOC & location \\
& MONEY & money \\
& NORP & nationality religion \\
& ORDINAL & ordinal \\
& ORG & organization \\
& PERCENT & percent \\
& PERSON & person \\
& PRODUCT & product \\
& QUANTITY & quantity \\
& TIME & time \\
& WORK\_OF\_ART & work of art \\

\bottomrule
\end{tabular}

}

\end{center}
\caption{Original labels and their corresponding natural-language-form type names of datasets under {Domain Transfer} settings.}
\label{tab:dataset_labels_nlf_2}
\end{table}

\subsubsection{Variant Type Names}\label{appendix_variant_type_names}
Tables~\ref{app:tab:variant_types_fewnerd} and~\ref{app:tab:variant_types_transfer} show the variant type names used in the analysis experiments on the impact of type names in Section~\ref{sec:impact_type_names}.

\begin{table*}[]
\small
\begin{center}
    \resizebox{\textwidth}{!}{
    \begin{tabular}{llll}
    \toprule
    \multicolumn{1}{l}{\textbf{Original Type Names}} & \multicolumn{1}{l}{\textbf{Synonym 1}} & \multicolumn{1}{l}{\textbf{Synonym 2}} & \multicolumn{1}{l}{\textbf{Synonym 3}} \\
    \cmidrule(lr){1-1} \cmidrule(lr){2-4}
    broadcast program                                & television show                        & TV program                             & telecast                               \\
    film                                             & movie                                  & motion picture                         & cinema                                 \\
    music                                            & melody                                 & tunes                                  & songs                                  \\
    other art                                        & different art                          & alternative art                        & diverse art                            \\
    painting                                         & artwork                                & canvas                                 & picture                                \\
    written art                                      & literature                             & written work                           & prose                                  \\
    actor                                            & performer                              & thespian                               & artist                                 \\
    artist author                                    & creative writer                        & author                                 & wordsmith                              \\
    athlete                                          & sportsman/woman                        & player                                 & competitor                             \\
    director                                         & filmmaker                              & supervisor                             & manager                                \\
    other person                                     & someone else                           & another person                         & another individual                     \\
    politician                                       & statesman/woman                        & lawmaker                               & public servant                         \\
    scholar                                          & academic                               & intellectual                           & researcher                             \\
    soldier                                          & military personnel                     & serviceman/woman                       & trooper                                \\
    airplane                                         & aircraft                               & plane                                  & jet                                    \\
    car                                              & automobile                             & nourishment                            & fare                                   \\
    food                                             & cuisine                                & nourishment                            & fare                                   \\
    game                                             & sport                                  & competition                            & match                                  \\
    other product                                    & different product                      & alternative item                       & various commodity                      \\
    ship                                             & vessel                                 & boat                                   & craft                                  \\
    software                                         & program                                & application                            & computer program                       \\
    train                                            & locomotive                             & railway vehicle                        & railcar                                \\
    weapon                                           & armament                               & firearm                                & arm                                    \\
    astronomy thing                                  & celestial object                       & astronomical entity                    & heavenly body                          \\
    award                                            & accolade                               & prize                                  & recognition                            \\
    biology-thing                                    & biological entity                      & living organism                        & life form                              \\
    chemical thing                                   & chemical substance                     & compound                               & element                                \\
    currency                                         & money                                  & cash                                   & legal tender                           \\
    disease                                          & illness                                & sickness                               & disorder                               \\
    educational degree                               & academic qualification                 & diploma                                & certification                          \\
    god                                              & deity                                  & divine being                           & higher power                           \\
    language                                         & tongue                                 & speech                                 & communication                          \\
    law                                              & legislation                            & legal system                           & jurisprudence                          \\
    living thing                                     & organism                               & creature                               & being                                  \\
    medical                                          & healthcare                             & medicinal                              & therapeutic                            \\
    bodies of water                                  & Waterways                              & aquatic features                       & lakes and rivers                       \\
    geographical social political entity             & Territory                              & region                                 & jurisdiction                           \\
    island                                           & Isle                                   & islet                                  & key                                    \\
    mountain                                         & Peak                                   & summit                                 & range                                  \\
    other location                                   & Site                                   & spot                                   & place                                  \\
    park                                             & Garden                                 & reserve                                & recreational area                      \\
    road railway highway transit                     & Route                                  & thoroughfare                           & transportation network                 \\
    company                                          & Corporation                            & firm                                   & enterprise                             \\
    education                                        & Learning                               & schooling                              & instruction                            \\
    government agency                                & Public body                            & administrative department              & authority                              \\
    media newspaper                                  & Press                                  & journalism                             & news organization                      \\
    other organization                               & Institution                            & establishment                          & association                            \\
    political party                                  & Political group                        & faction                                & party organization                     \\
    religion                                         & Faith                                  & belief system                          & spirituality                           \\
    show organization                                & Production company                     & entertainment group                    & performance troupe                     \\
    sports league                                    & Athletic association                   & sporting federation                    & league organization                    \\
    sports team                                      & Athletic club                          & competitive squad                      & sporting roster                        \\
    \bottomrule
    \end{tabular}
    }
\end{center}
\caption{Variant type names for Few-NERD Intra setting.}
\label{app:tab:variant_types_fewnerd}
\end{table*}

\newpage

\begin{table*}[]
\small
\begin{center}
    {
    \begin{tabular}{llll}
    \toprule
    \multicolumn{1}{l}{\textbf{Original Type Names}} & \multicolumn{1}{l}{\textbf{Synonym 1}} & \multicolumn{1}{l}{\textbf{Synonym 2}} & \multicolumn{1}{l}{\textbf{Synonym 3}} \\
    \cmidrule(lr){1-1} \cmidrule(lr){2-4}
    cardinal                                         & Primary                                & fundamental                            & principal                              \\
    date                                             & Day                                    & time                                   & appointment                            \\
    event                                            & Occasion                               & happening                              & function                               \\
    fac                                              & Facility                               & building                               & structure                              \\
    geographical social political entity             & Territory                              & region                                 & jurisdiction                           \\
    language                                         & Tongue                                 & speech                                 & communication                          \\
    law                                              & Regulation                             & rule                                   & statute                                \\
    location                                         & Place                                  & site                                   & spot                                   \\
    money                                            & Currency                               & funds                                  & finances                               \\
    nationality religion                             & Citizenship                            & faith                                  & belief system                          \\
    ordinal                                          & Sequential                             & numbered                               & ordered                                \\
    organization                                     & Institution                            & establishment                          & association                            \\
    percent                                          & Percentage                             & proportion                             & rate                                   \\
    person                                           & Individual                             & human                                  & character                              \\
    product                                          & Item                                   & good                                   & merchandise                            \\
    quantity                                         & Amount                                 & volume                                 & measure                                \\
    time                                             & Duration                               & period                                 & interval                               \\
    work of art                                      & Artwork                                & creation                               & masterpiece                            \\
    \midrule
    \midrule
    person                                           & Individual                             & human being                            & somebody                               \\
    location                                         & Place                                  & site                                   & spot                                   \\
    organization                                     & Institution                            & establishment                          & company                                \\
    miscellaneous                                    & Various                                & diverse                                & mixed                                  \\
    \bottomrule
    \end{tabular}
    }
\end{center}
\caption{Variant type names for Domain Transfer setting. Here we show the type names in the OntoNotes dataset and the CoNLL2003 dataset.}
\label{app:tab:variant_types_transfer}
\end{table*}
